# Supplementary material for: Detection of Illicit Drug Trafficking Events on Instagram: A Deep Multimodal Multilabel Learning Approach
Source: arXiv:2108.08920 source file (2021-08-23)
Supplement: Supplementary file 1 [file appendix.tex]

\newpage
\appendix

\section{Reproducibility}

More details about data
